# Supplementary material for: A melting mode of frozen sessile droplets with unmelted ice layer deposited at the bottom
Source: arXiv:2602.08803 source file (2026-02-09)
Supplement: Supplementary file 1 [file MeltingBottom_SM.pdf]

# A melting mode of frozen sessile droplets with unmelted ice layer deposited at the bottom: Supplementary Materials

Jiawang Cui,[1] Yugang Zhao,[2] Tianyou Wang,[1,3] and Zhizhao Che*[1,3]

[1)]*State Key Laboratory of Engines, Tianjin University, Tianjin, 300350, China.*

[2)]*Shanghai Key Laboratory of Multiphase Flow and Heat Transfer in Power Engineering, School of Energy and Power Engineering, University of Shanghai for Science and Technology, Shanghai 200093, China.*

[3)]*National Industry-Education Platform of Energy Storage, Tianjin University, Tianjin, 300350, China.*

(*Electronic mail: corresponding author: chezhizhao@tju.edu.cn)

(Dated: 5 December 2025)

## S1. EXPERIMENTAL DETAILS

### S1.1. Experimental setup and procedure

The experimental setup consists of a freezing part and a melting part, which is similar to our previous study[1], as shown in Figures S1(a) and S1(b), respectively. The freezing part was used to freeze droplets on substrates, and the melting part to control and observe the melting process of the frozen droplets. Throughout the experiment, the substrate surface temperatures were maintained using a semiconductor temperature control system for both processes. As for the solid substrates in the experiment, a silicon wafer was used as the experimental substrate of superhydrophobic surfaces, and it has a small thickness of 0.7 mm and a high thermal conductivity of 148 W/(m·K). A clean and flat copper plate with a thickness of 1 mm was also selected as the experimental substrate, which has a high thermal conductivity of 401 W/(m·K). Therefore, the temperature of the experimental substrate could quickly reach the setting value to melt the frozen droplet.

In the experiment, the substrate was initially positioned on the copper plate of the freezing part, which was maintained at a temperature of -20 °C. Then, droplets of different volumes were placed on this cold substrate through a needle. Upon completion of supercooling, nucleation, and freezing, the frozen droplet and its substrate were transferred to the melting part and deposited on the preheated copper plate for the melting study after the copper plate was heated to a melting temperature required for the experiment. The droplet morphology during melting was captured by a CMOS camera (FLIR BFS-U3-17S7M-C) with a macro lens (TOKINA AT-X PRO 100 mm), while illumination was provided by an LED light source. To visualize the flow pattern during the melting, fluorescent polystyrene microspheres (Thermo Fisher R0300, mean diameter 3 $\mu$m) were added to the water at a concentration of $7.6 \times 10^3$ particles/$\mu$L. The density of polystyrene ($\sim$ 1.05 g/cm$^3$) is close to that of water, so the particles are nearly neutrally buoyant. Because of their small size, the corresponding settling velocity is negligible over the melting time scale (tens of seconds), and preliminary tests confirmed that the presence of particles does not measurably affect the melting time or the evolution of the ice-water interface.

In all experiments, the droplet volume was chosen in the range of several tens of microliters. A volume of 37.1 $\mu$L was used on the HMN and SN superhydrophobic substrates, while droplet volumes of up to 55.6 $\mu$L were used on the Cu substrate to reach its maximum apparent contact angle. This range ensures that the droplets remain in the sessile, surface-tension-dominated regime.

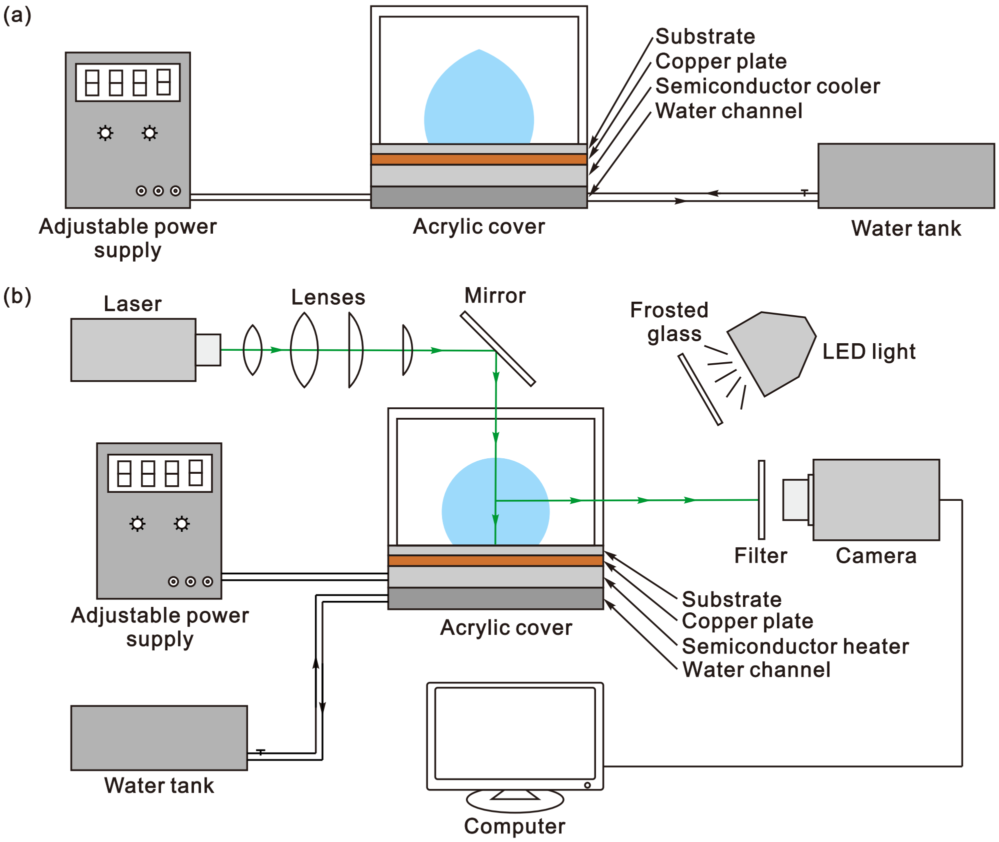


FIG. S1. Schematic diagram of the experimental setup: (a) droplet freezing experiment; (b) droplet melting experiment.

Within this volume range, the melting mode (floating and deposited) is primarily controlled by contact angle, heating temperature, and particle concentration, while the droplet volume mainly affects the total melting time and the size of the lubrication film.

## S1.2. Experimental substrates

In the experiment, three kinds of substrates with different surface characteristics were used to study their effect on melting droplets, as shown in Figure S2. Micro/nanostructures were created on silicon wafers to produce two types of superhydrophobic surfaces. One superhydrophobic substrate was fabricated by applying a uniform PDMS coating to a silicon wafer. Hydrophobic silica powder was then evenly distributed across the surface and secured through vibrational settling into the PDMS layer. Following thermal curing, the surface exhibited a static water contact angle of 153°. This kind of superhydrophobic surface was named hierarchical-scale micro-nano-structured

(HMN) superhydrophobic substrate, as shown in Figure S2(a). The other superhydrophobic substrate was fabricated by spray-coating a homogeneous solution (composed of fluororesin, butyl acetate, and fluorinated silica, with a solid content of 12%) on the silicon wafer. After drying, silica particles were stacked on the substrate, creating a superhydrophobic surface with a static contact angle of 162°. This kind of superhydrophobic surface was named single-scale nano-structured (SN) superhydrophobic substrate, as shown in Figure S2(b). In addition, a smooth, unmodified copper plate (1 mm thick) is used as the third substrate type for comparative analysis, as shown in Figure S2(c). To make the droplet on the unmodified copper surface in an apparently hydrophobic state, circular grooves were fabricated on the copper surface to constrain the expansion of the three-phase contact line of the droplet, resulting in the droplet presenting a maximum apparent contact angle of 132°.

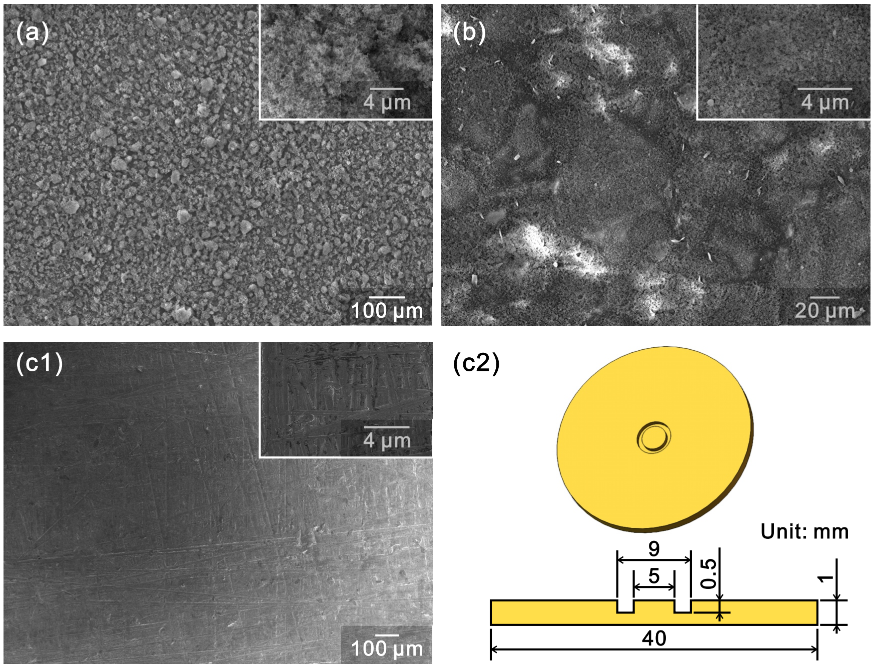


FIG. S2. Three types of substrates used in this study: (a) SEM images of the hierarchical-scale micro-nano-structured (HMN) superhydrophobic substrate; (b) SEM images of the single-scale nano-structured (SN) superhydrophobic substrate; (c) SEM images and geometric model of the Cu substrate.

## S2. CHARACTERISTICS OF THE MELTING PROCESS

### S2.1. Melting flow

The overlaid particle trajectories in Figure 3 can be used as a qualitative visualization of the internal flow pattern and relative flow intensity in the melting droplet. Due to the three-dimensional geometry and optical distortions near the water-air interface, a fully quantitative PIV/PTV analysis of the velocity distribution is beyond the scope of the present study. On the HMN substrate, there are two regular flow vortices within the melting droplet. In contrast, for the melting process on the SN substrate, the flow intensity in the melted area is much weaker than that on the HMN substrate, and regular flow can only be seen near the left/right sides of the unmelted ice layer. For the formation of the regular flow, due to the deposition of an unmelted ice layer downward, the melted fluid between the ice layer and the heating wall is squeezed and gradually expelled via the side of the droplet. For the effect of overall weak flow, the top of the unmelted ice layer remains almost unchanged, especially in the early stage. In general, the flow can affect the morphology of the unmelted ice layer and its melting speed.

### S2.2. Melting morphology

According to the experimental results shown in Figure 1, the contact angle and heating temperature affect the path and intensity of heat transfer between the unmelted ice layer and the heated wall, respectively. Therefore, the contact angle and the heating temperature affect the temperature distribution inside the droplet, indirectly changing the flow inside the droplet, and ultimately affecting the morphology of the unmelted ice layer.

The influence of the apparent contact angle on the morphology of the unmelted ice layer is experimentally examined as shown in Figure S3(a). The apparent contact angle is adjusted by controlling the volume of droplets on the Cu substrate, that is, the aspect ratio of the droplet is altered. During the initial stage of melting, there are two approaches of heat transfer. One approach is to transfer heat between the unmelted ice layer and the heating wall through thermal conduction, mainly near the central area of the droplet, where there is almost no flow. The other approach of heat transfer between the unmelted ice layer and the heated wall is through thermal convection, mainly near the gas-liquid interface of the droplet, where Marangoni convection exists. For a droplet with a small apparent contact angle, the droplet is relatively wide. The melted area caused

by the two approaches of heat transfer has no clear boundary, because the bottom of the unmelted ice layer is almost horizontal, as shown in Figure S3(a1). For a droplet with a large apparent contact angle, the droplet is relatively tall. The melted areas caused by the two approaches of heat transfer have a clear edge, as shown in Figure S3(a2). The area from the bottom of the two corners of the unmelted ice layer to the heating wall is due to thermal conduction, while the area between the bottom corner of the unmelted ice layer and the gas-liquid interface of the droplet is caused by thermal convection. In general, increasing the contact angle of droplets can affect the morphology of the unmelted ice layer.

The influence of heating temperature on the change of unmelted ice layer morphology is experimentally examined and shown in Figure S3(b). Due to the presence of an unmelted ice layer, temperature gradients within the melted fluid induce dual convective mechanisms: natural convection originating from thermally induced density change and Marangoni convection stemming from temperature-dependent surface tension variation. The natural convection and Marangoni convection result in different melting speeds at different parts of the ice layer. For the melting process on the HMN substrate, Marangoni convection dominates the flow, leading to rapid melting at the sides and slow melting at the bottom. Therefore, with increasing heating temperature, the maximum height of the melted area at the sides increases (note that the comparison for different conditions is based on the moment when the bottom of the unmelted ice layer reaches the same height). It means that a higher heating temperature promotes the flow in the droplet, especially on the sides of the droplet where the Marangoni convection originates, thereby enhancing the heat and mass transfer in these areas. Therefore, the heating temperature is an important factor that can alter the morphology of the unmelted ice layer.

Although temperature gradients in the melted liquid generate both natural convection and Marangoni convection, the deposited mode arises in a Marangoni-dominated regime, where strong interfacial shear drives melted water above the ice layer and a thin lubrication film forms at the ice-substrate interface. Natural convection primarily affects the global temperature and velocity fields during melting. As the relative strength of Marangoni convection decreases and becomes comparable to natural convection, the deposited configuration loses stability and the unmelted ice layer transitions to the floating mode.

Because the micro/nano-structures on the surfaces of superhydrophobic substrates are often fragile, especially in the process of freezing, particles may detach from the superhydrophobic substrate and enter the droplet. The particles can change the flow in the droplet and affect the

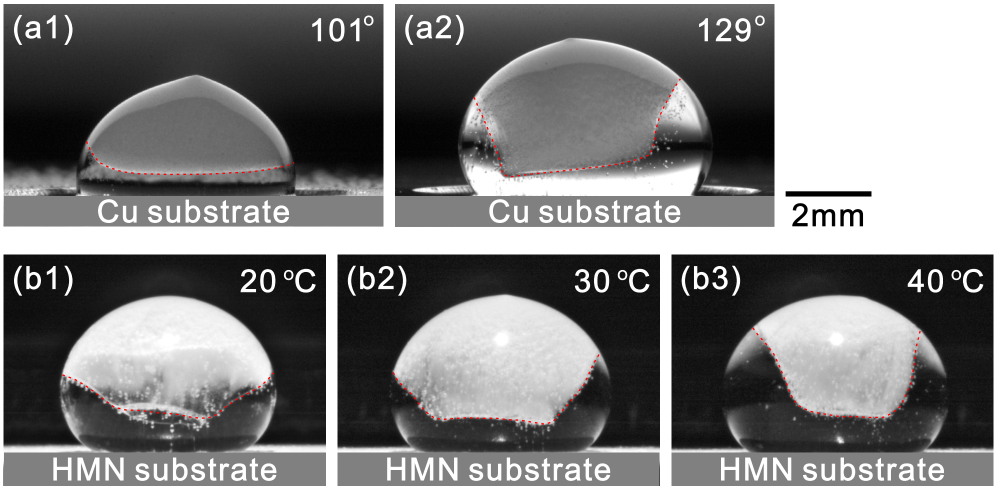


FIG. S3. Morphology of the unmelted ice layer on the (a) Cu and (b) HMN substrates at different apparent contact angles and heating temperatures, respectively. The heating temperature is 30 °C in Figure S3(a), and the droplet volume is 37.1 $\mu$l in Figure S3(b).

morphology of the unmelted ice layer. Therefore, the effect of particles on the melting process is explored in Figure S4. Due to the randomness of the particle detachment from superhydrophobic surfaces in the freezing/melting process, here, to accurately control the influence of particles, particles were added into the droplet at different concentrations before the deposition of the droplet on the Cu substrate. Monodispersed silica microspheres with an average diameter of 500 nm were used and were evenly dispersed into the droplet. Because the distribution of particles at the gas-liquid interface has an inhibitory effect on the Marangoni convection[2], the flow near the surface of the droplet becomes much weaker than that of pure water droplets. During the experiment, the melting flow is dominated by Marangoni convection, at least within the range of particle concentration considered in this study. In this condition of melting, the bottom of the unmelted ice layer gradually becomes flatter with the increase in the particle concentration, which means that the melting flow intensity gradually decreases. This indicates a gradual reduction of the difference in the melting speed between the side and the bottom of the unmelted ice layer. For example, the unmelted ice layer at $t = 19$ s in Figure S4(a) has a nearly vertical side and two bottom corners of approximately 90°. This shape is in contrast to those at higher particle concentrations, for example, $t = 18$ s in Figure S4(b) and at $t = 20$ s in Figure S4(c). Therefore, the particle concentration can affect the morphology of the unmelted ice layer by changing the flow intensity, which is also the reason for the difference in the melting processes between the HMN substrate and SN substrate

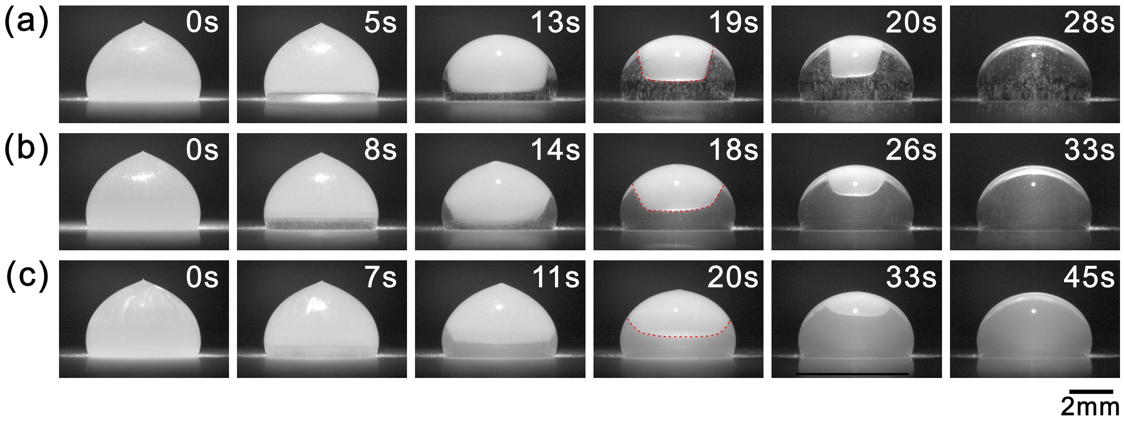


FIG. S4. Morphology of the unmelted ice layer on the Cu substrate at different concentrations of monodispersed silica microspheres: (a) $2.5 \times 10^{-6}$ g/ml; (b) $1.7 \times 10^{-4}$ g/ml; (c) 8.3 $\times 10^{-4}$ g/ml. The heating temperature is 40 °C, and the droplet volume is 55.6 $\mu$l.

at the same heating temperature (see Section S4 of the Supplementary Material).

## S3. TRANSITION OF THE MELTING MODE

The intensity of flow under different heating temperatures directly affects the melting mode, but the intensity of flow may change during the melting process, which may affect the interfacial forces on the unmelted ice layer and then alter the melting mode. The melting process of a frozen droplet on the SN substrate under the heating temperature of 25 °C (as shown in Figure S5) is an example of the transition in the melting mode. According to the shape and position of the unmelted ice layer, the melting process in this condition can be categorized into four distinct stages. In Stage I, the unmelted ice layer is located at the top of the droplet. Two narrow melted zones are on the sides of the droplet due to the Marangoni convection, and a thin melted zone is at the bottom of the melting droplet due to the thermal conduction from the heating wall. All of these are not affected by the subsequent melting mode. In Stage II, the unmelted ice layer tightly adheres to the bottom of the droplet as the melting process progresses (i.e., the deposited mode); In Stage III, the unmelted ice layer quickly rises to the top of the droplet, during which the unmelted ice layer may shake and flip. Finally, in Stage IV, the unmelted ice layer stays at the top of the droplet as the melting process progresses (i.e., the floating mode). Why do the two melting modes exist in the same melting process, and why does the deposited mode exist before the occurrence of the floating mode but not after? According to our previous study[1], the intensity of the melting flow

inside the droplet dominated by the Marangoni convection gradually decreases with the melting process because of the decrease in the differences in intensity between the Marangoni convection and natural convection. When the flow at the gas-liquid interface is strong enough to quickly achieve a sufficient amount of melted fluid at the top of the ice layer, the unmelted ice layer will move to the top of the droplet under the effect of buoyancy. Thus, the melting mode changes from the deposited mode to the floating mode and cannot change back to the deposited mode. The transition of the melting mode can be achieved due to the variation of the flow intensity during the same melting process, as long as the intensity of the Marangoni convection is similar to that of natural convection at a certain moment. In our experiment, we only observed the transition from the deposited mode to the floating mode of the ice cap, but did not observe the transition from the floating mode to the deposited mode. This is mainly because the ice cap floating on the top is more stable than deposited at the bottom, and the buoyancy force determines the final mode of the melting process.

The energy analysis reveals that the variation in melting flow characteristics during mode transition accounts for the significant disparity in melting times between the two regimes. As shown in Figures S3(a) and S3(b), the intensity of the melting flow in the floating mode is much greater than that in the deposited mode. Even in the same melting process, the intensity of the melting flow at the end of Stage III (the floating mode, see Figure S5(c)) is much greater than that at the beginning of Stage III (the deposited mode, see Figure S5(b)), although the time between these two instants is only a few seconds. In the floating mode, the thermal energy transferred from the substrate promotes the flow inside the droplet, thereby increasing the average temperature of the melted fluid and then accelerating the heat exchange between the melted fluid and the unmelted ice layer. While in the deposited mode, the thermal energy transferred from the substrate promotes the flow at the gas-liquid interface to maintain the unmelted ice layer deposited at the bottom of the droplet. Because the fluid generated after melting immediately flows to the area above the ice layer, although a stable low-temperature side (i.e., the interface between melted water and unmelted ice) exists, there is no significant temperature gradient within this area due to the lack of a stable high-temperature side (i.e., the fluid temperature is more uniform) and is difficult to induce flow. Throughout the melting process, most thermal energy from the substrate is used to melt the ice (except for the heat losses in the system, e.g., dissipation to the environment). Moreover, the thermal contact resistance at the ice-substrate interface in deposited mode is substantially lower than observed in floating mode configurations. Therefore, the deposited mode has more

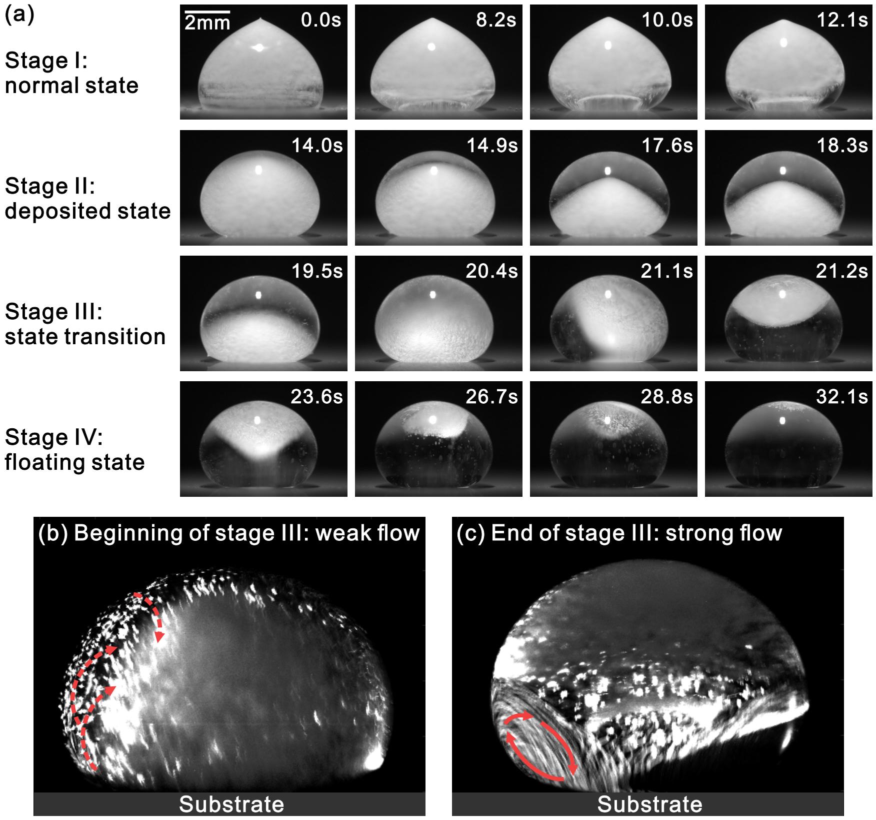


FIG. S5. Melting process of a frozen droplet on the SN substrate. The experiment is conducted with a fixed heating temperature of 30 °C and a controlled droplet volume of 37.1 $\mu$l. (a) Four stages of the melting process are divided according to the characteristics of the unmelted ice layer. At stage I, the droplet is in a normal state. The melting occurs on both sides and at the bottom of the melting droplet, and there is no significant difference regardless of the subsequent melting mode. At stage II, the unmelted ice layer is in a deposited state, while at stage IV, the unmelted ice layer is in a floating state. As for stage III, the unmelted ice layer can be transferred from the bottom to the top of the droplet in just a few seconds, achieving the transition of the melting mode. (b) Melting flow in the droplet at the beginning of stage III. (c) Melting flow in the droplet at the end of stage III. A video clip for the melting process is available as the Supplementary Material.

advantages from the perspective of promoting droplet melting, such as in de-icing applications.

## S4. CONDITIONS FOR THE DEPOSITED MODE

What is the condition for the deposition of the unmelted ice layer at the bottom during the melting process? Through the analysis of the effects of contact angle, heating temperature, and

particle concentration on the melting process in Section S2.2 of the Supplementary Material, it has been shown that the pattern and intensity of the melting flow affect the morphology of the unmelted ice layer. By increasing the heating temperature and reducing the inhibitory effect of particles, the intensity of flow can be increased, resulting in more fluid flowing to the top of the unmelted ice layer. It should be noted that simply increasing the intensity of the flow trend is not enough for the transition from the floating mode to the deposited mode. The unmelted ice layer's morphology exhibits significant dependence on the contact angle. As shown in Figure 2a, the melting processes of frozen droplets on the Cu substrate (with a maximum contact angle of 132°, much lower than that of the superhydrophobic substrates) at the heating temperatures from 20 to 80 °C were experimentally tested, and the deposited mode did not occur. In this condition, although the intensity of flow has been guaranteed by high heating temperature and no particle inhibition, the deposited mode does not occur because a narrow flow area is formed, which can guide the melted liquid to the top of the unmelted ice layer. The failure to achieve the deposited mode on the Cu substrate can be attributed to the shape of the droplet on the substrate, which is determined by the contact angle. For droplets on substrates with small contact angles, the extensive interfacial contact between the droplet and heated substrate promotes significant melting beneath the ice layer. The large melted area causes the melted fluid at the gas-liquid interface to flow toward the area with lower flow resistance (i.e., under the unmelted ice layer) rather than to the top of the unmelted ice layer, which leads to insufficient force to make the unmelted ice layer move downward. In contrast, for droplets on substrates with large contact angles, their aspect ratio allows for melting at the bottom while forming narrow melted areas on both sides (as shown in Figure S3(a) of the Supplementary Material). This narrow shape makes it difficult for the melted fluid at the gas-liquid interface to flow downward, and then the melted fluid can only flow toward the top of the unmelted ice layer. Therefore, the shape of the droplet is an important factor for the melting model, and a large contact angle is necessary for the droplet to achieve the deposited mode. In addition, the stable deposition of unmelted ice layer requires a certain flow velocity within the liquid film. Therefore, the Marangoni effect on both sides of the droplet should have a certain strength to guide the melted fluid out. In general, a high flow intensity and narrow flow area at the gas-liquid interface of a melting droplet are important for the deposition of the unmelted ice layer at the bottom. All of these can make more melted fluid move upward to realize the deposited melting mode.

Based on the above analysis, the fact that the SN substrate exhibits the deposited mode at lower

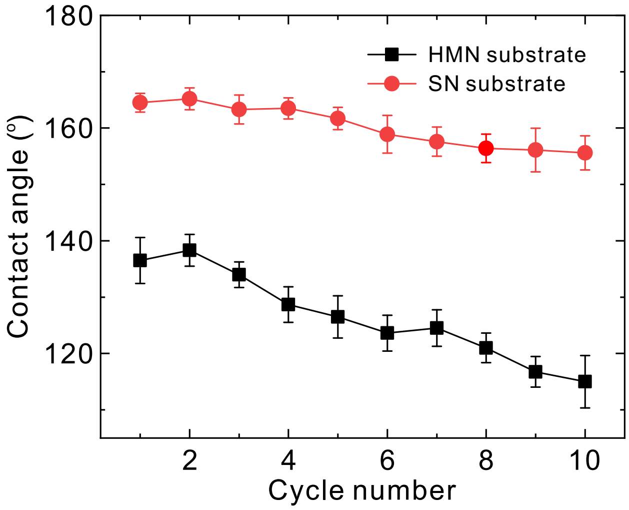


FIG. S6. Contact angle of the droplet after each complete melting on the HMN and SN substrates during cycled freezing-melting processes. The heating temperature is 30 °C, and the droplet volume is 43.6 $\mu$l.

heating temperatures than the HMN substrate (Figure 2a) results from a combination of factors. First, the micro/nano-structures on the SN surface are more robust, causing less particle detachment during repeated freezing-melting cycles; the weaker particle-induced damping of Marangoni convection leads to stronger interfacial flow along the gas–liquid interface. Second, the SN substrate has a slightly higher static contact angle (162° vs. 153° on HMN), which increases the droplet aspect ratio and narrows the lateral melted regions at the sides of the ice layer. These geometric changes favor the upward transport of melted water above the ice layer and thereby facilitate the deposited mode.

As for the difference in the melting processes between the HMN substrate and SN substrate at the same heating temperature (e.g., 30 °C), it can be attributed to the influence of particle detachment from these superhydrophobic surfaces. The delicate nature of superhydrophobic micro/nanostructures renders them susceptible to degradation under repeated freezing and melting processes[3]. Surface durability can be quantitatively evaluated through systematic contact angle measurements, where decreasing values after each freezing-melting cycle correlate with progressive damage to the superhydrophobic structures. In Figure S6, after experiencing multiple freezing and melting cycles, there is a relatively small decrease in the contact angle on the SN substrate compared with that on the HMN substrate. This means that the macro/micro-structures on the SN substrate can better maintain their integrity during the freezing-melting processes. With less detachment of particles, the inhibition effect of the particles on the melting flow is relatively weaker. Therefore, with

a stronger interfacial flow and a larger contact angle on the SN substrate, it is more probable for the unmelted ice layer to be deposited at the bottom of the melting droplet.

## REFERENCES

[1]J. Cui, T. Wang, and Z. Che, "Melting process of frozen sessile droplets on superhydrophobic surfaces," Langmuir **39**, 14800–14810 (2023).

[2]F. Du, L. Zhang, and W. Shen, "The internal flow in an evaporating human blood plasma drop," Journal Colloid and Interface Science **609**, 170–178 (2022).

[3]J. Feng, Y. Pang, Z. Qin, R. Ma, and S. Yao, "Why condensate drops can spontaneously move away on some superhydrophobic surfaces but not on others," ACS Applied Materials & Interfaces **4**, 6618–6625 (2012).
